# Supplementary material for: Kramers nodal line in the charge density wave state of YTe$_3$ and the influence of twin domains
Source: arXiv:2405.10222 source file (2024-05-16)
Supplement: Supplementary file 1 [file YTe3_arpes_dft_SM_arXiv.pdf]

# Supplementary information for "Kramers nodal line in the charge density wave state of $YTe_3$ and the influence of twin domains"

Shuvam Sarkar[1*], Joydipto Bhattacharya[2,3], Pramod Bhakuni[1], Pampa Sadhukhan[1], Rajib Batabyal[1], Christos D. Malliakas[4], Marco Bianchi[5], Davide Curcio[5], Shubhankar Roy[6], Arnab Pariari[7], Vasant G. Sathe[1], Prabhat Mandal[7], Mercouri G. Kanatzidis[4,8], Philip Hofmann[5], Aparna Chakrabarti[2,3], Sudipta Roy Barman[1†]

[1]*UGC-DAE Consortium for Scientific Research, Khandwa Road, Indore 452001, Madhya Pradesh, India*

[2]*Theory and Simulations Laboratory, Raja Ramanna Centre for Advanced Technology, Indore 452013, Madhya Pradesh, India*

[3]*Homi Bhabha National Institute, Training School Complex, Anushakti Nagar, Mumbai 400094, Maharashtra, India*

[4]*Department of Chemistry, Northwestern University, Evanston, 60208, Illinois, USA*

[5]*Department of Physics and Astronomy, Interdisciplinary Nanoscience Center (iNANO), Aarhus University, 8000 Aarhus C, Denmark*

[6]*Vidyasagar Metropolitan College, 39 Sankar Ghosh Lane, Kolkata 700006, India*

[7]*Saha Institute of Nuclear Physics, HBNI, 1/AF Bidhannagar, Kolkata 700 064, India and*

[8]*Materials Science Division, Argonne National Laboratory, Lemont, Illinois 60439, USA*

TABLE S1. Crystal data and structure refinement for $YTe_3$ at 100 K.

| | |
|---|---|
| Empirical formula | $YTe_3$ |
| Formula weight | 471.7 |
| Temperature | 100 K |
| Wavelength | 0.70926 Å |
| Crystal system | orthorhombic |
| Space group | C2cm(00$\gamma$)000 |
| Unit cell dimensions (in conventional setting) | a= 4.2840(7)Å, $\alpha$= 90°<br>b= 25.312(4)Å, $\beta$= 90°<br>c= 4.2932(9)Å, $\gamma$= 90° |
| q-vector(1) | 0.2907(4)c* |
| Volume | 465.54(15) Å$^3$ |
| Z | 4 |
| Density (calculated) | 6.728 g/cm$^3$ |
| Absorption coefficient | 31.041 mm$^{-1}$ |
| F(000) | 780 |
| $\theta$ range for data collection | 1.61 to 29.25° |
| Index ranges | $-5\leq h\leq 5$, $-34\leq k\leq 34$, $-6\leq l\leq 6$, $-1\leq m\leq 1$ |
| Reflections collected | 6556 |
| Independent reflections | 1937 [$R_{int}$ = 0.0558] |
| Completeness to $\theta$ = 29.25° | 98% |
| Refinement method | Full-matrix least-squares on $F^2$ |
| Goodness-of-fit on $F^2$ | 1.53 |
| Final R indices [I>2$\sigma$(I)] | $R_{obs}$ = 0.0365, w$R_{obs}$ = 0.0976 |
| R indices [all data] | $R_{all}$ = 0.0545, w$R_{all}$ = 0.1020 |
| Extinction coefficient | 0.00060(8) |
| Largest diff. peak and hole | 1.93 and -2.27 e·Å$^{-3}$ |

$R = \Sigma||F_o|-|F_c||/\Sigma|F_o|$, $wR = \{\Sigma[w(|F_o|^2-|F_c|^2)^2]/\Sigma[w(|F_o|^4)]\}^{1/2}$ and $w=1/(\sigma^2(I)+0.0016I^2)$

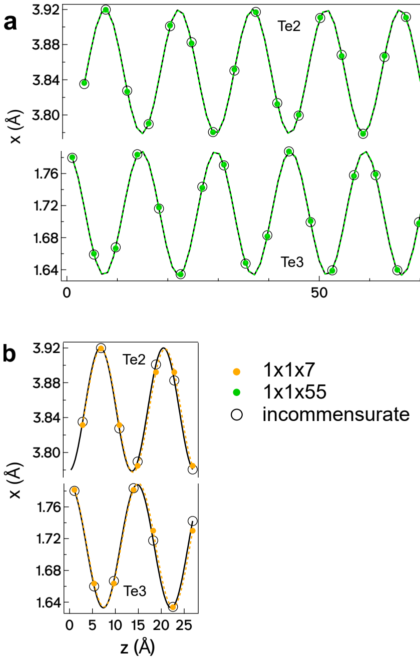


FIG. S1. Comparison of the Te (Te2 and Te3) atom positions in the $x$ direction between the incommensurate structure obtained from x-ray crystallography with (a) the 55-fold (55f) and (b) the 7-fold (7f) structure. $q_{\rm CDW}$ determined from a sinusoidal fit for the x-ray crystallography structure matches with the 55f structure (0.2909c*). The amplitude and the phase of the modulation wave are indistinguishable between the two and the atom positions almost coincide. On the other hand, for the 7f structure small differences are visible, as mentioned in the main text.

### A. Discussion: Evolution of the CDW gap across the Brillouin zone

To study the evolution of the CDW gap across the BZ, $E(k_z)$ cuts measured at different $k_x$ momenta are shown in Figs. S2(a-d); the measurement directions are indicated by blue horizontal lines on the right axis of Fig. 2(b). The corresponding 2D curvature plots are shown in Figs. S2(e-h). In Figs. S2(i-l), the calculated EBS are shown, where the influence of twin domains is accounted for by overlaying the EBS calculated along $k_x$ and $k_z$ directions for similar $k_z$ and $k_x$ momenta, respectively. In this way, an excellent agreement between the EBS and the ARPES bands is obtained. For example, the band involved in the CDW gap [indicated by the red arrow in Fig. S2(e)] is related to the domain *1* [indicated by the black dashed curves in Figs. S2(e,i)]. On the other hand, the other set of bands crossing the $E_F$ [indicated by blue arrow in Fig. S2(e)] are from domain *2* [blue bands in Fig. S2(i)]. Consequently, towards the BZ boundary with increasing $k_x$, we find that the bands related

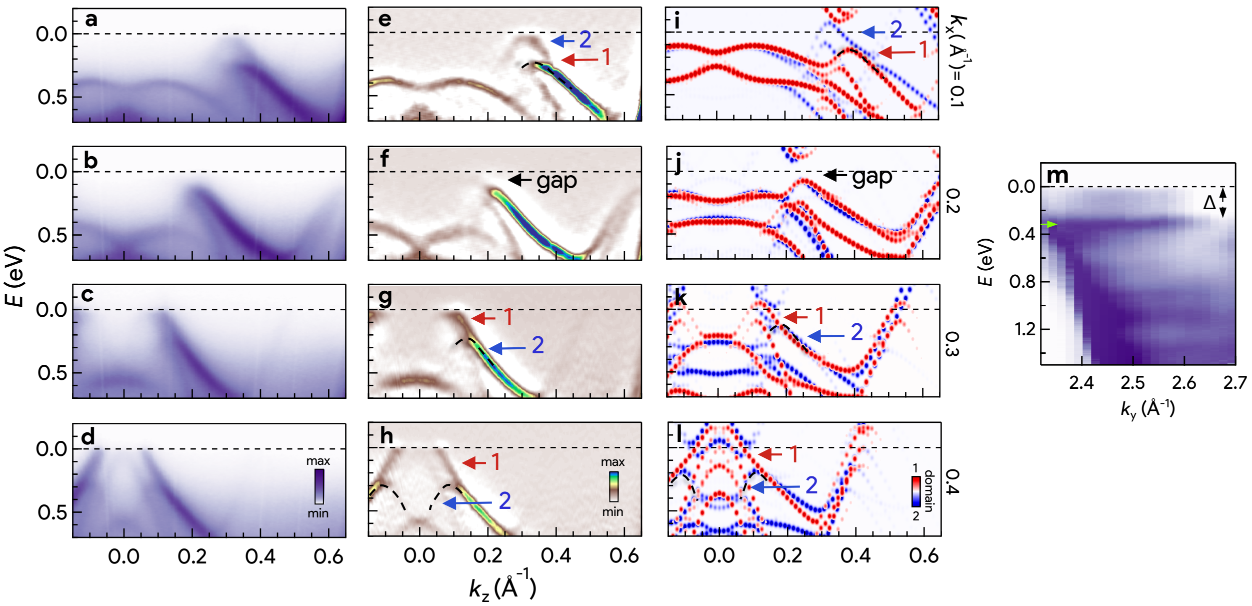


FIG. S2. (a-d) The $E(k_z)$ ARPES intensity plots at different $k_x$ values [cuts are indicated by blue lines on the right axis of Fig. 2(b)]. The color scale is shown as inset of panel **d**. (e-h) Curvature plots of panels **a-d**, respectively. The red and blue arrows indicate the bands related to domain *1* and *2*, respectively. The color scale is shown as inset of panel **h**. (i-l) The corresponding EBSs calculated at different $k_x$ portraying the CDW gap variation. The black dashed curves, indicating the band dispersion, are shown as guide to the eye. The color scale is shown as inset of panel **l**. (m) The $E(k_y)$ ARPES intensity plot measured using photon energy dependent scan (h$\nu$= 16-30 eV with 0.05 eV step) at $k_{||}$= 0.61 Å$^{-1}$.

to domain *1* closes the CDW gap [see the red bands in Figs. S2(i-l)] and cross the $E_F$ at $k_x$= 0.3 Å$^{-1}$[Fig. S2(g)]. On the contrary, the domain *2* bands [black dashed curves in Figs. S2(g,h) and (k,l)] move towards higher $E$ with increasing CDW gap towards larger $k_x$. This is because for domain *2*, the $\Gamma Z$ direction is approached. Interestingly, only at $k_x$= 0.2 Å$^{-1}$, we find that both the bands of the two domains show a CDW gap of $\Delta$ ∼0.15 eV [black arrows in Figs. S2(f) and (j)]. This shows that the narrow gapped part of the FS around $k_x$ of 0.2 Å$^{-1}$ in the $\alpha$ sheet is related to the CDW gap [red arrow in Fig. 2(b)]. Note that the value of $\Delta$ at $k_x$= 0.2 Å$^{-1}$ is smaller in comparison to the $\Gamma Z$ direction [$k_x$= 0, as shown in Fig. 2(b)]. This observation is in agreement with with the $k_x$-dependence previously reported by Brouet *et al.* [1].

The CDW gap along the perpendicular direction to $k_x$-$k_z$ plane is studied by an $E(k_y)$

cut at $k_{||}$= 0.61 Å$^{-1}$ [cut #1 shown by red arrow in Fig. 2(f)] in Fig. S2(m). This set of ARPES measurements has been performed by varying the photon energy (see methods). It shows that the occupied band (green arrow) that determines the CDW gap does not disperse, suggesting the CDW gap to be unchanged along $k_y$. In fact, three other bands that appear between $E$= 0.9 to 1.4 eV have almost no dependence on the $k_y$, suggesting a quasi-2D nature of these bands. In fact, based on this we argue that the FS measured with 24-28 eV is a close representation of the FS on the Γ plane.

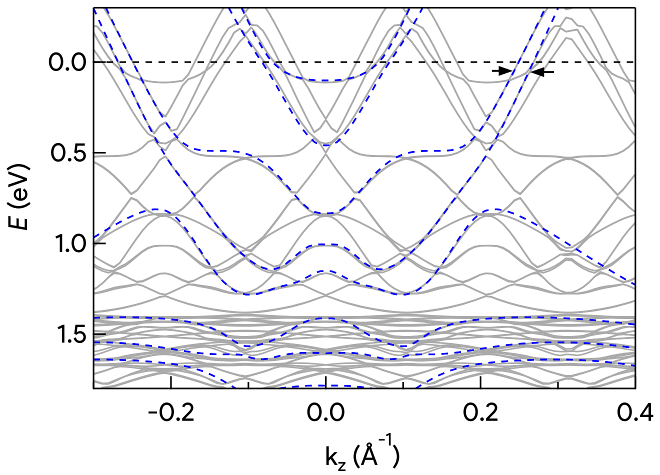


FIG. S3. The folded band structure of $YTe_3$ in the CDW state, calculated along $k_z$ at $k_x$= 0.59 Å$^{-1}$(gray curves). The blue dashed curves representing non-CDW bands are overlaid onto the CDW bands. A pair of black arrows indicates that the bilayer splitting is similar between CDW and non-CDW state.

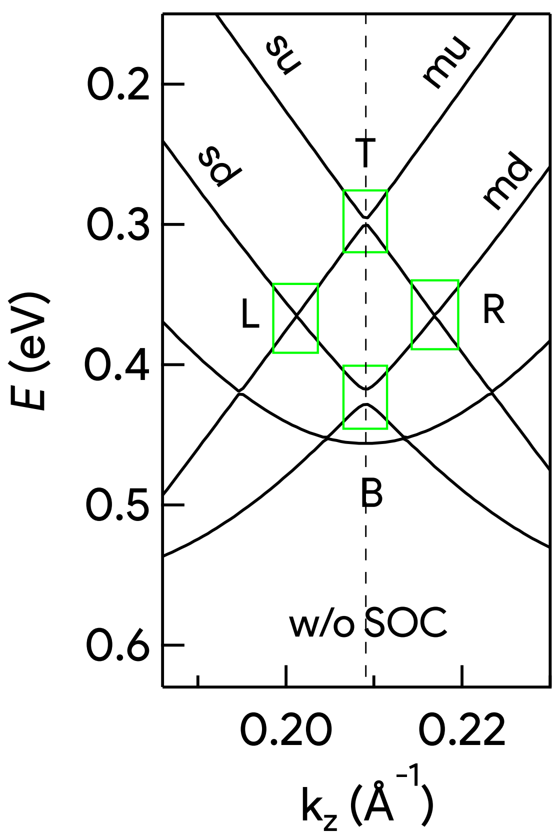


FIG. S4. $E(\mathrm{k}_z)$ folded bands without SOC at $\mathrm{k}_x$= 0.59 Å$^{-1}$ in the crossing region of the main and shadow bands. The vertical dashed line represents the $\mathrm{k}_z$ point on $\Gamma_2 X_2$ i.e., the $\Sigma$ line in the second BZ [see Fig. 2(a) of the main text].

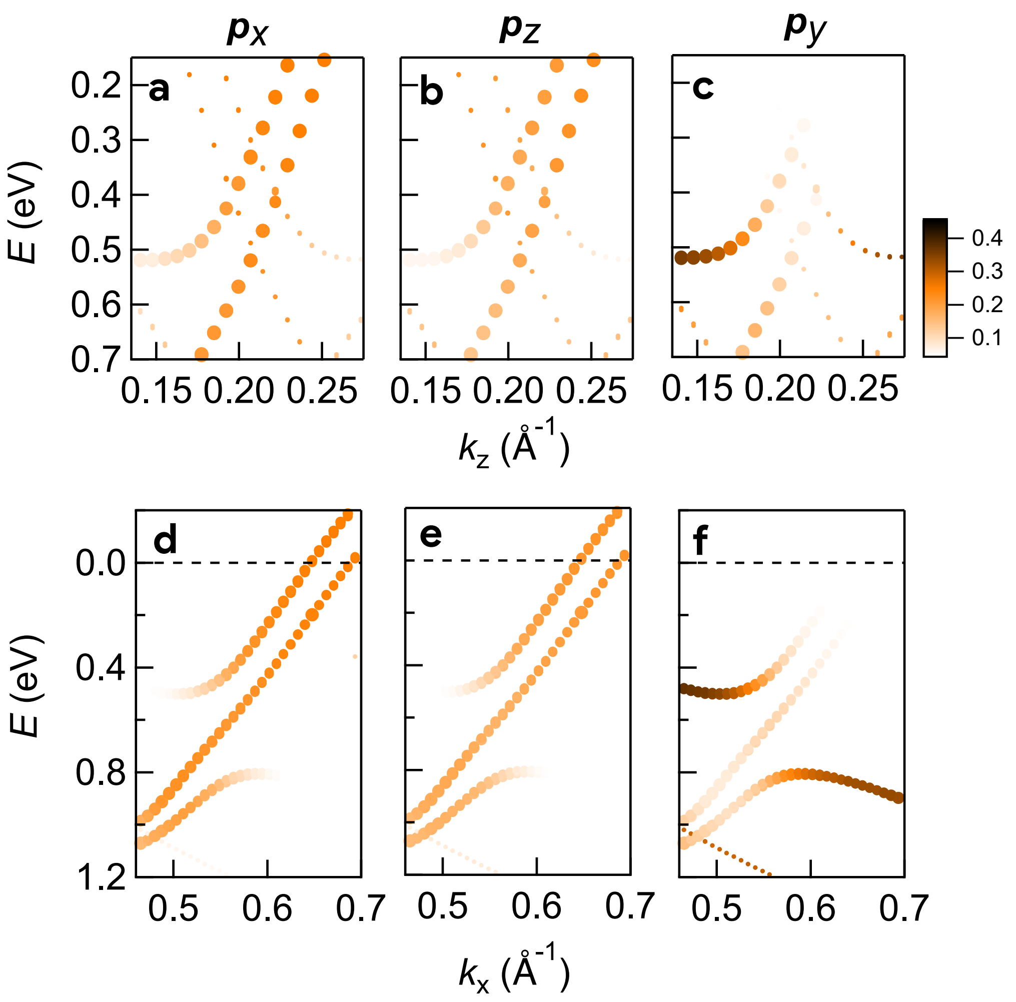


FIG. S5. The Te $p_x$, $p_z$ and $p_y$ orbital characters of the EBS (a-c) along $k_z$ at $k_x$= 0.59 Å$^{-1}$near the crossing region and (d-f) along $k_x$ at $k_z$= 0.209 Å$^{-1}$ (i.e., $\Gamma_2 X_2$), the corresponding EBS is shown in panel **f** of Fig. 4. The size and the intensity of the markers indicate the unfolded weights and the orbital characters, respectively. The color scale for all panels is shown in the right side of panel **c**, where the values show the orbital contribution.

[1] V. Brouet, W. L. Yang, X. J. Zhou, Z. Hussain, R. G. Moore, R. He, D. H. Lu, Z. X. Shen, J. Laverock, S. B. Dugdale, N. Ru, and I. R. Fisher, Phys. Rev. B **77**, 235104 (2008).
